# Supplementary material for: Pixel is a Barrier: Diffusion Models Are More Adversarially Robust Than We Think
Source: arXiv:2404.13320 source file (2024-05-02)
Supplement: Supplementary file 1 [file pdm_pure_ablation.pdf]

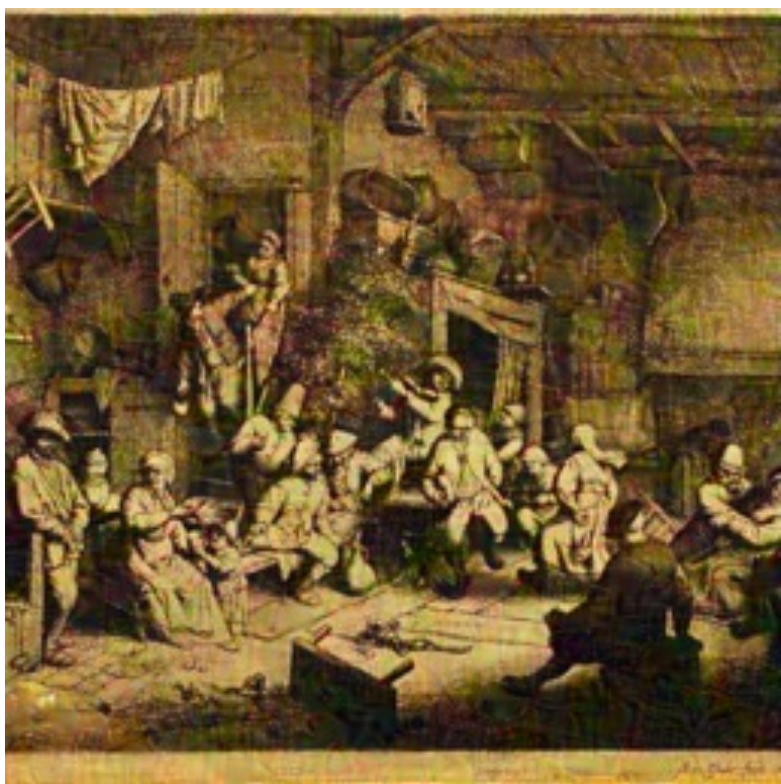

Protected  
AdvDM

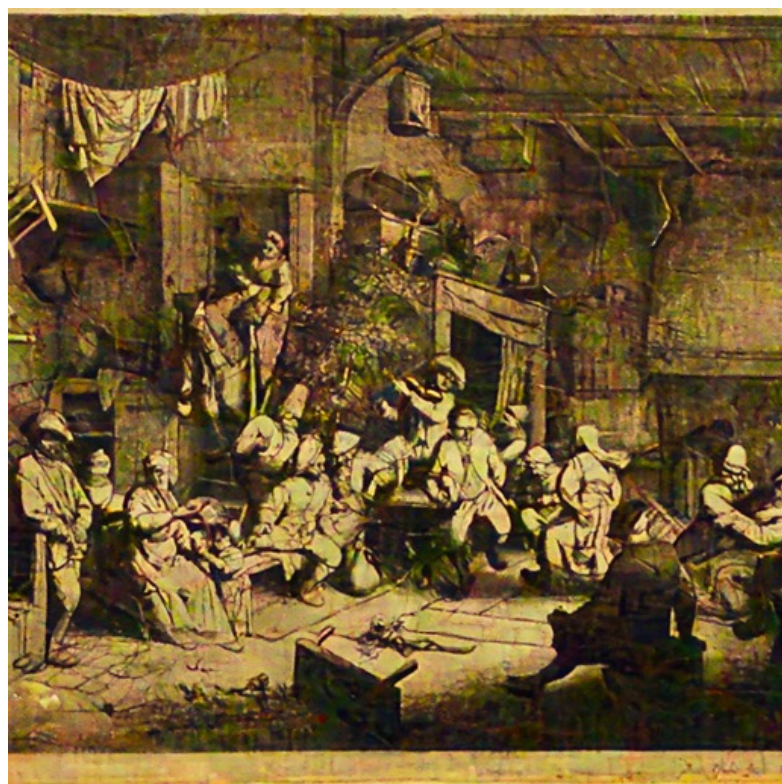

PDM-Pure  
( $t^* = 0.01$ )

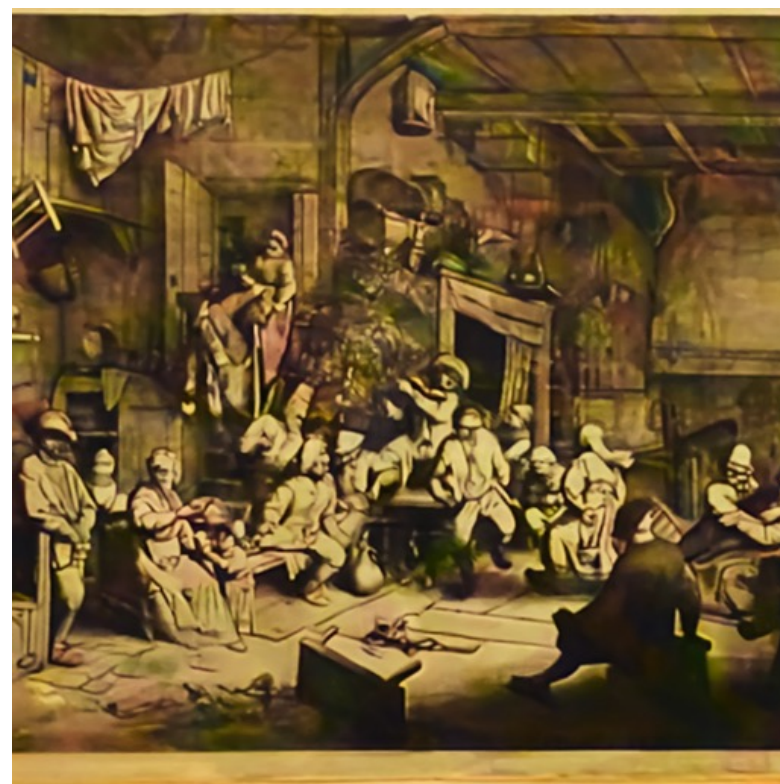

PDM-Pure  
( $t^* = 0.1$ )

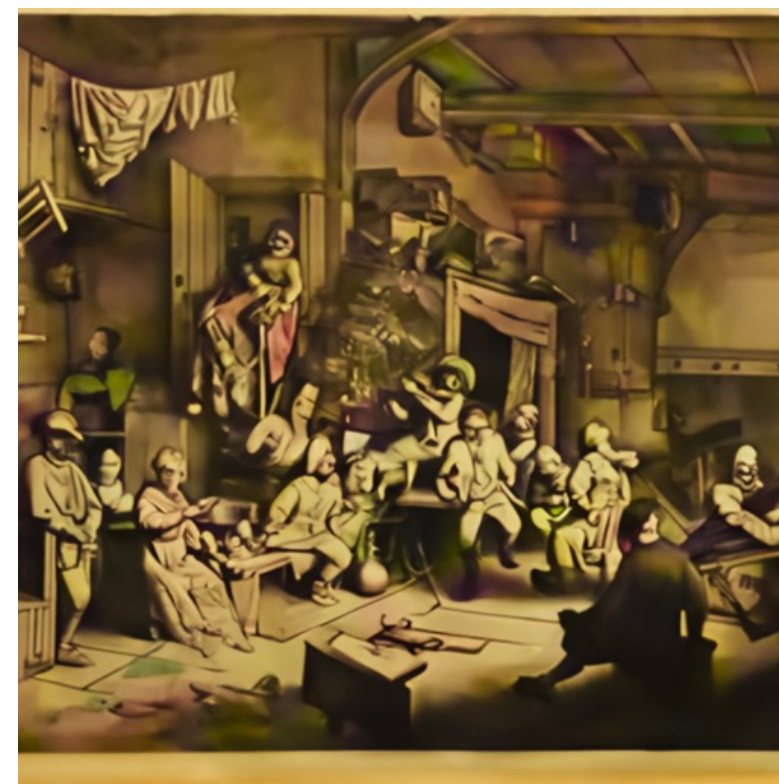

PDM-Pure  
( $t^* = 0.2$ )

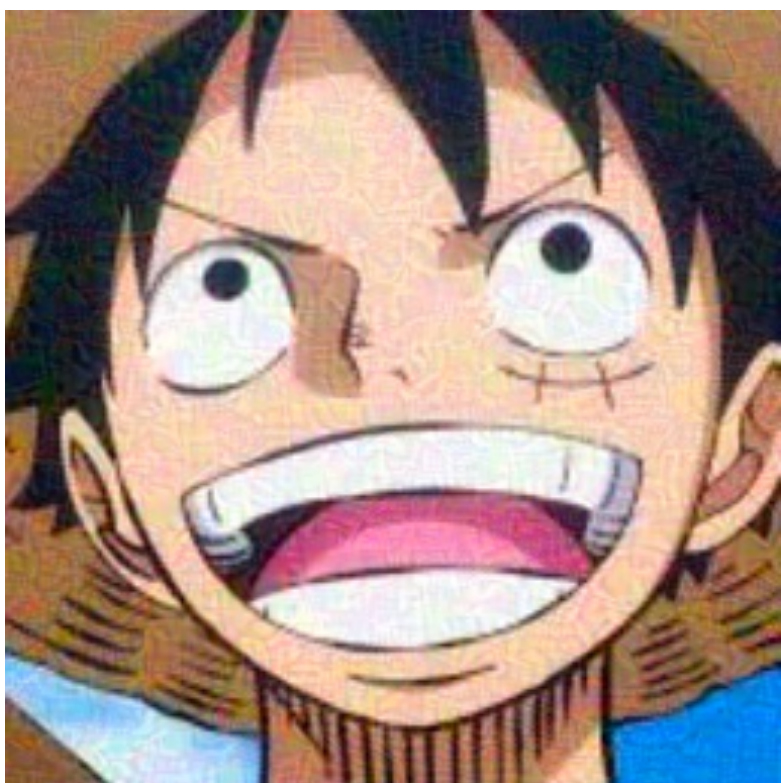

Protected  
AdvDM

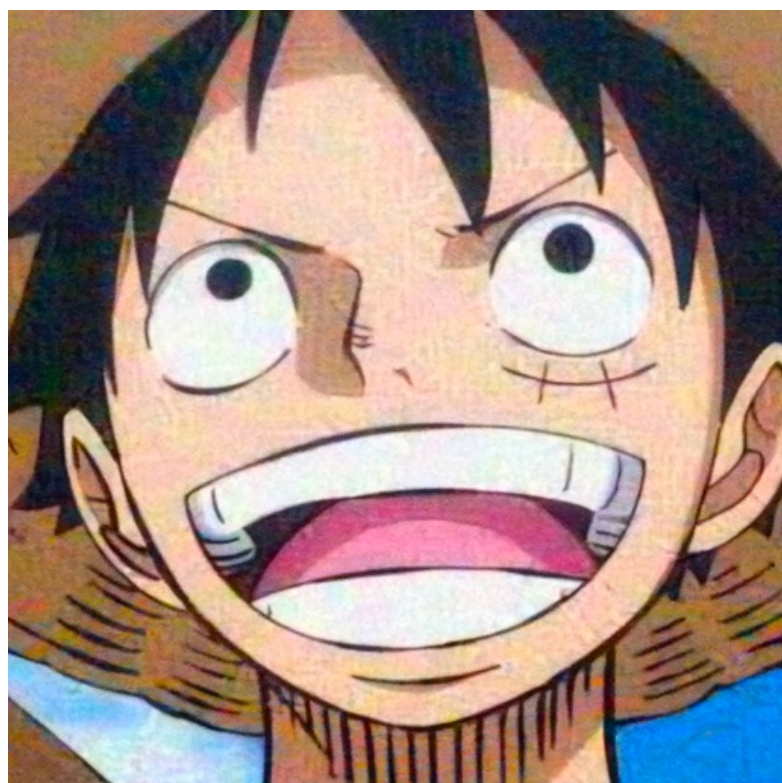

PDM-Pure  
( $t^* = 0.01$ )

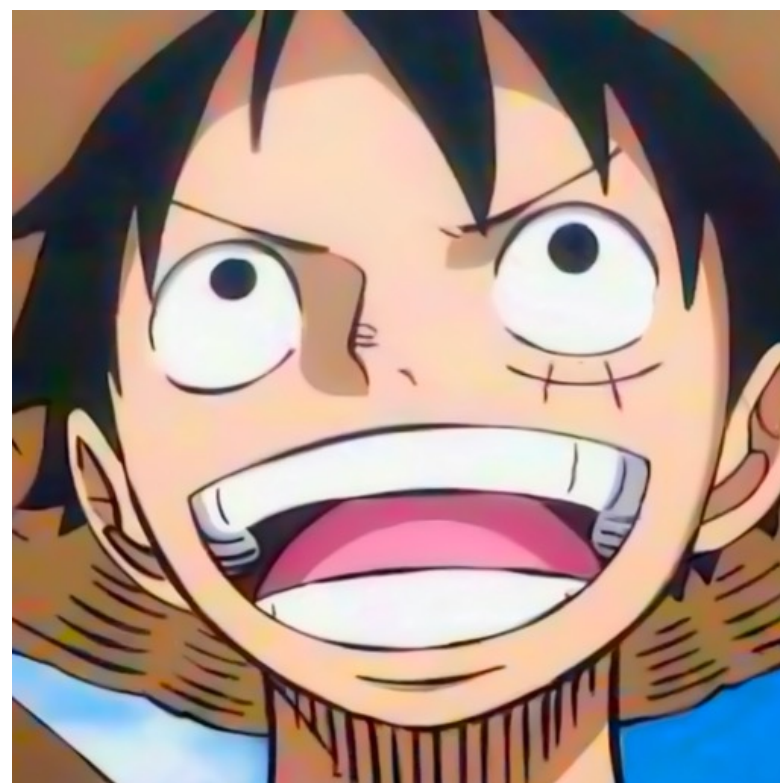

PDM-Pure  
( $t^* = 0.1$ )

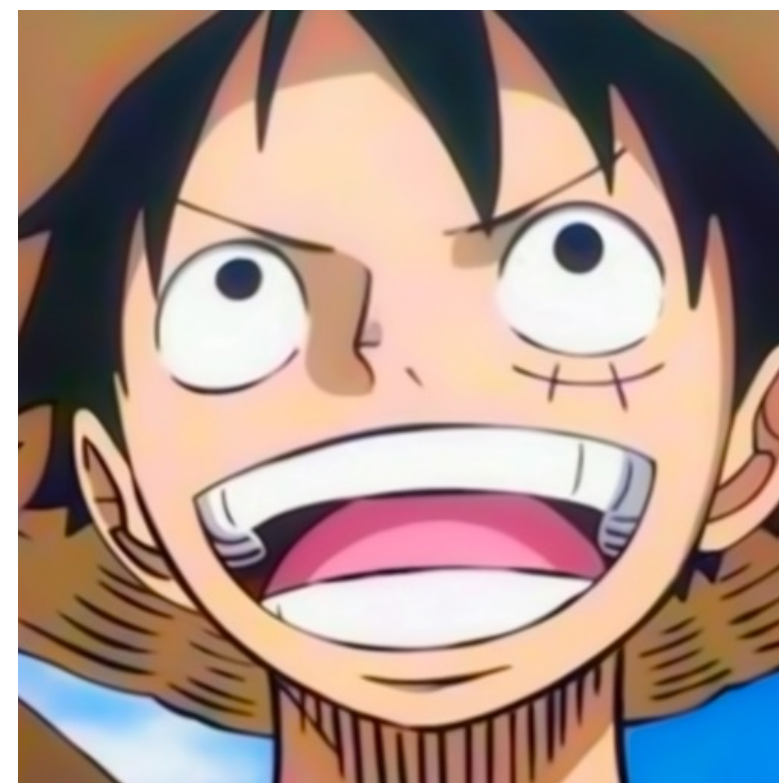

PDM-Pure  
( $t^* = 0.2$ )

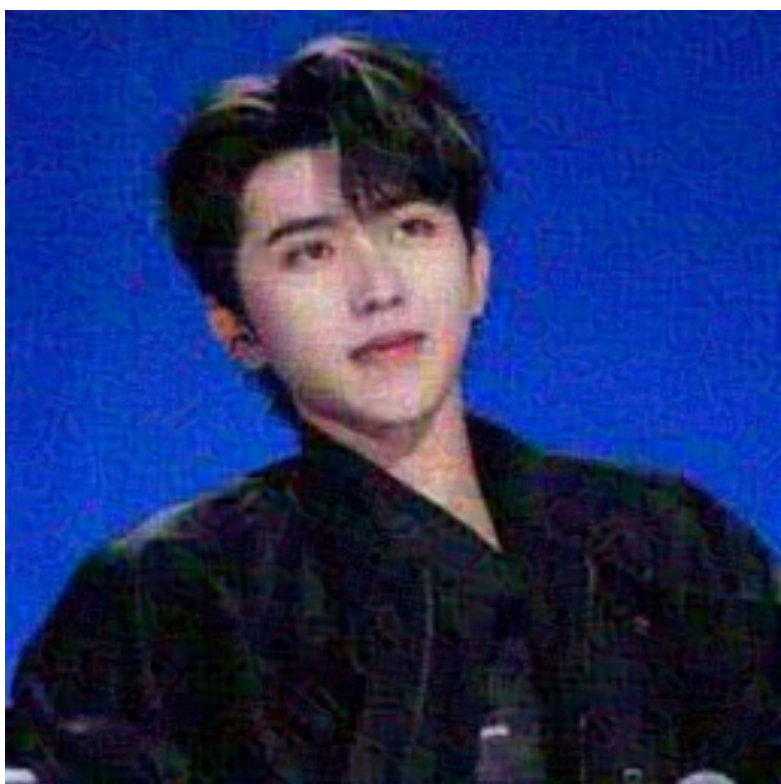

Protected  
AdvDM

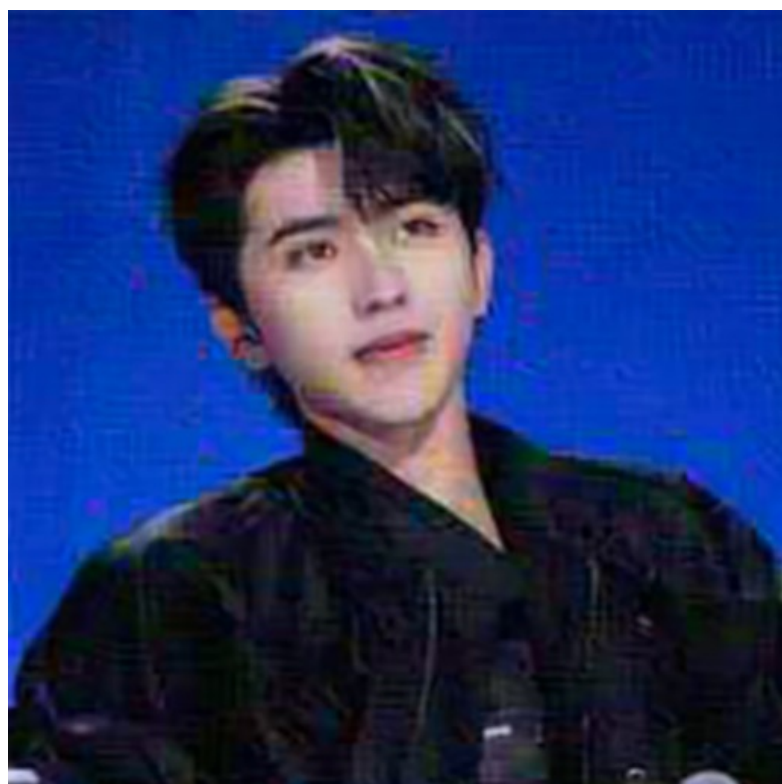

PDM-Pure  
( $t^* = 0.01$ )

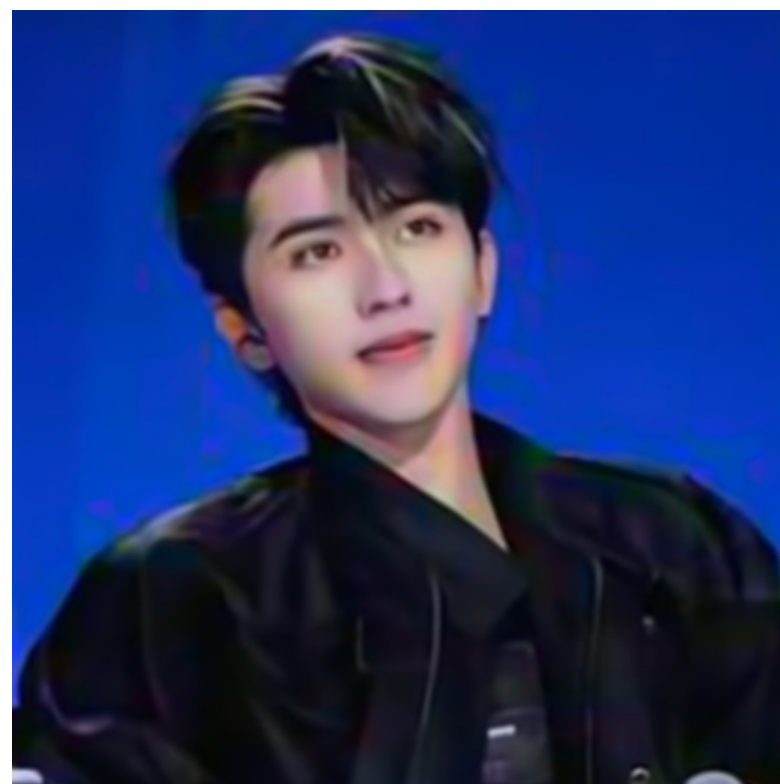

PDM-Pure  
( $t^* = 0.1$ )

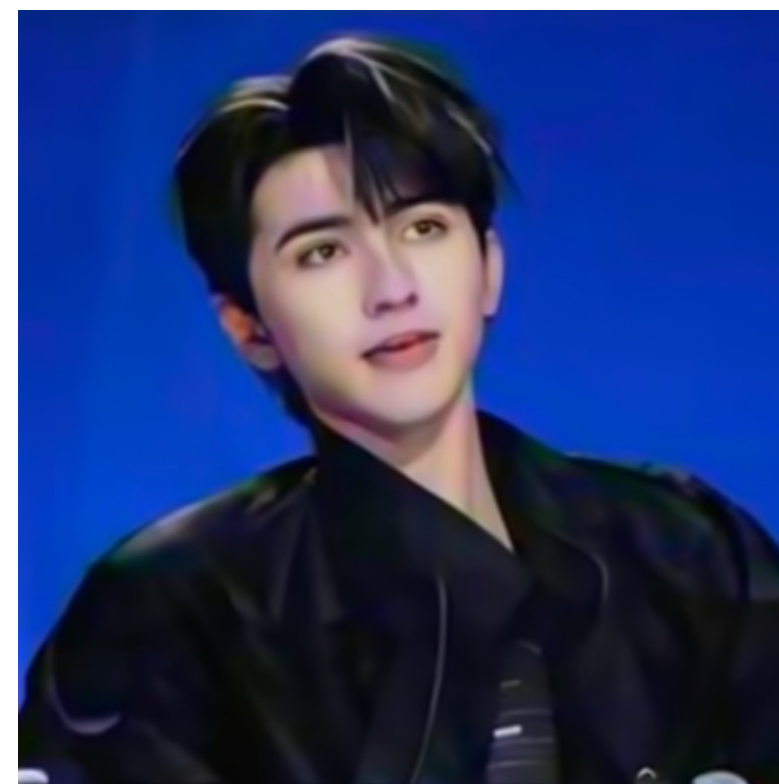

PDM-Pure  
( $t^* = 0.2$ )

Mist

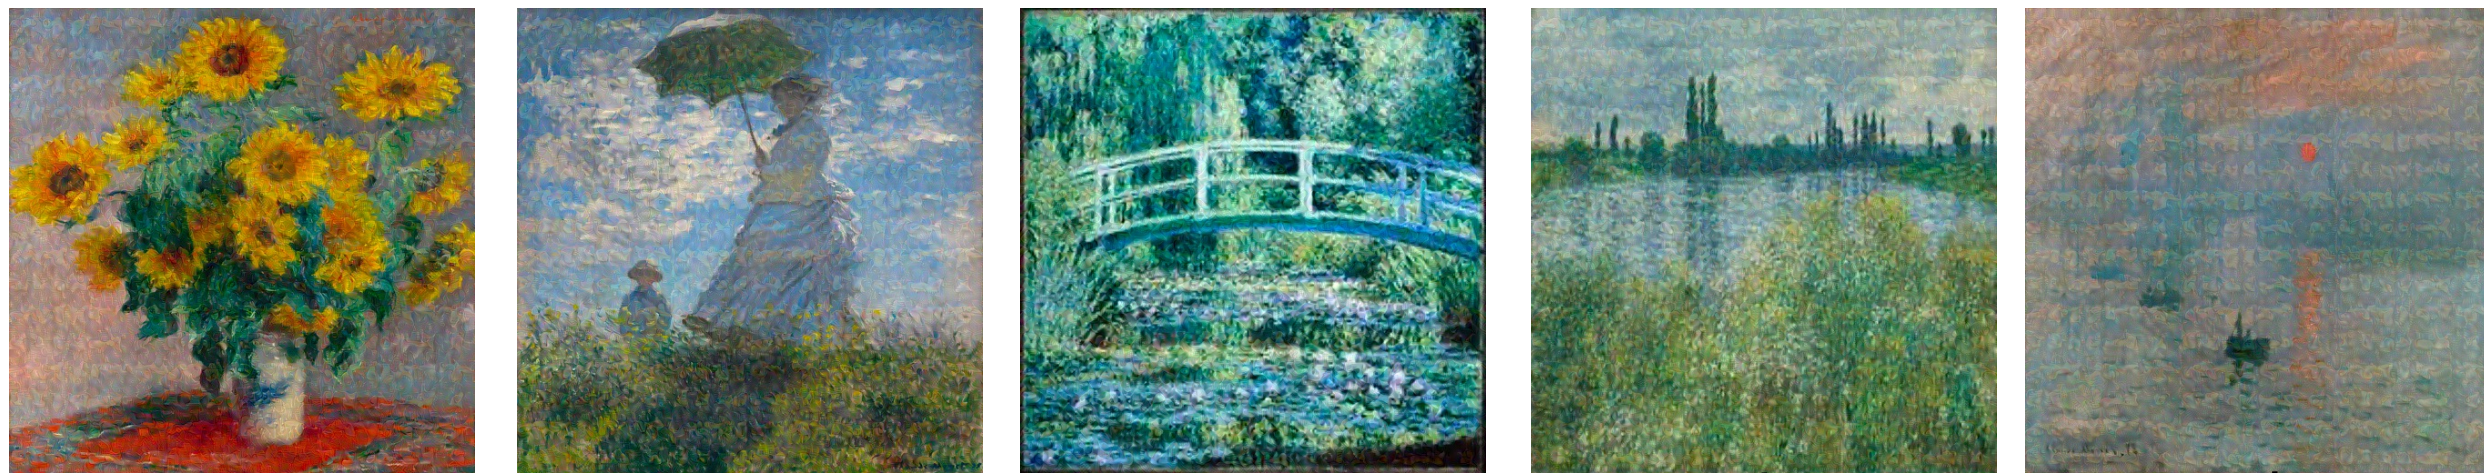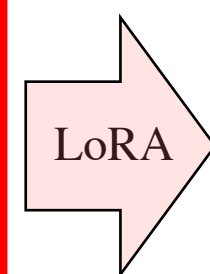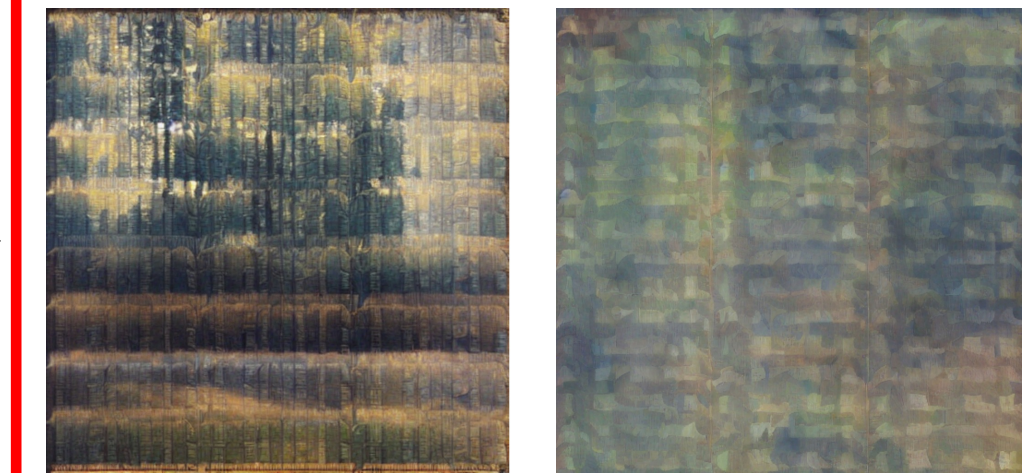

Prompt: 'a painting of a forest'

PDM-Pure

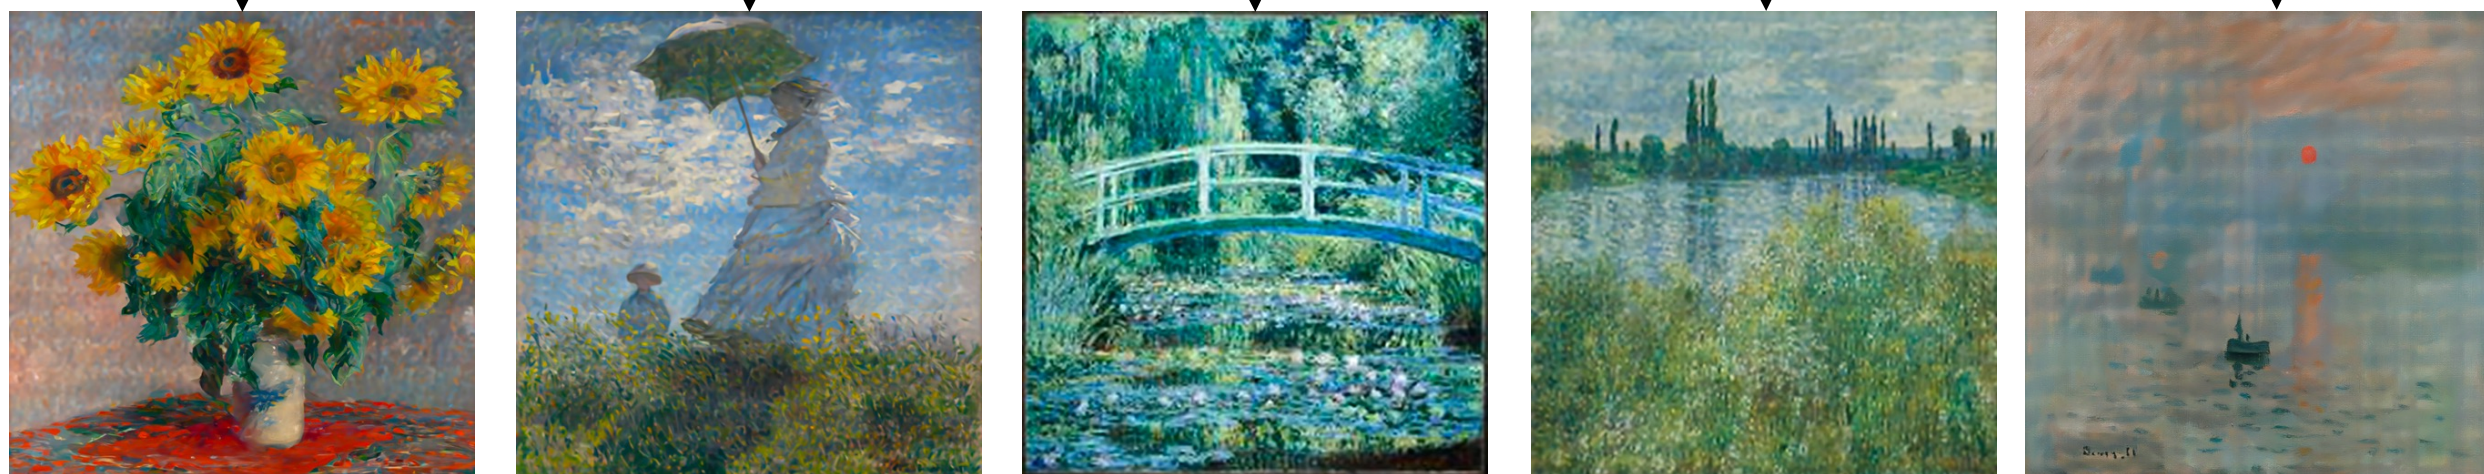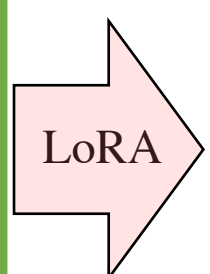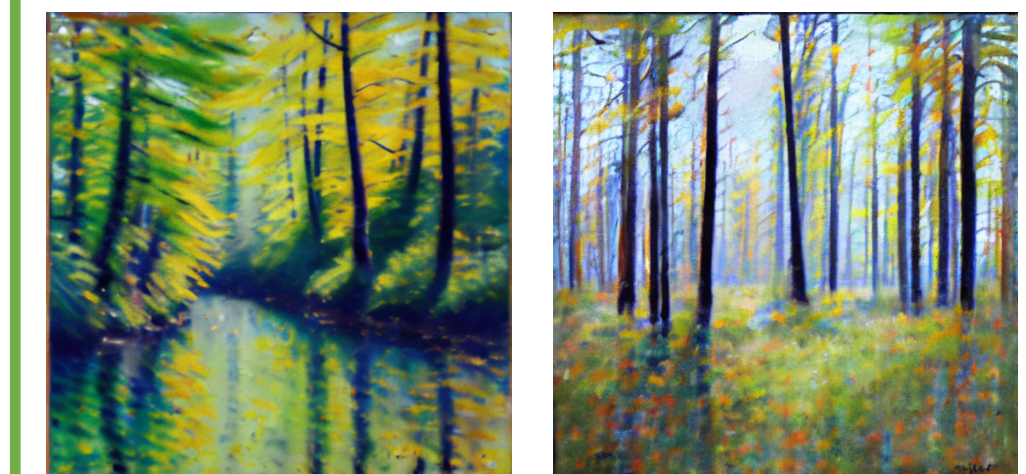

Prompt: 'a painting of a forest'

Glaze

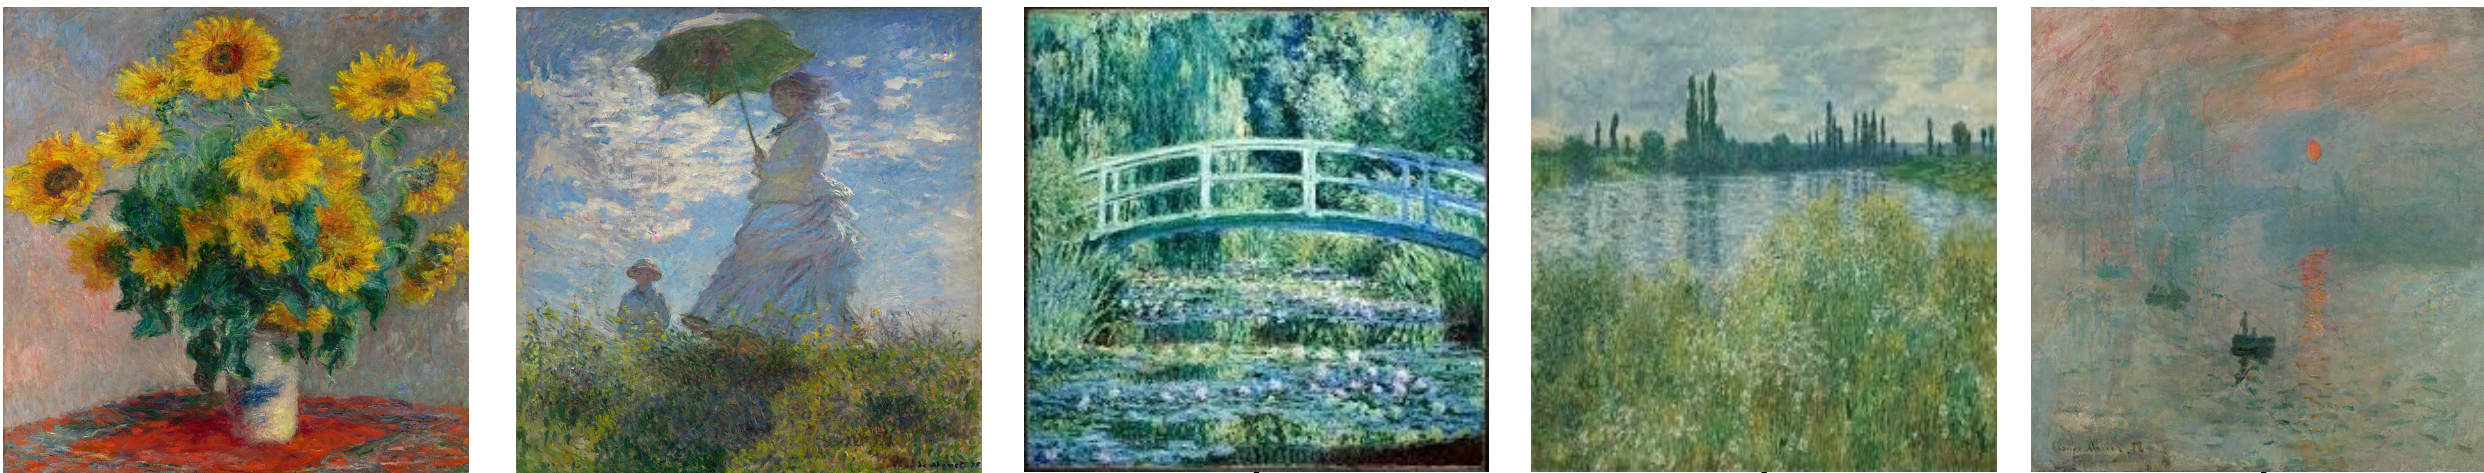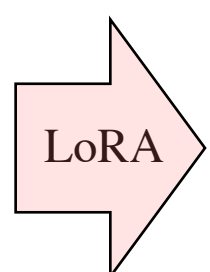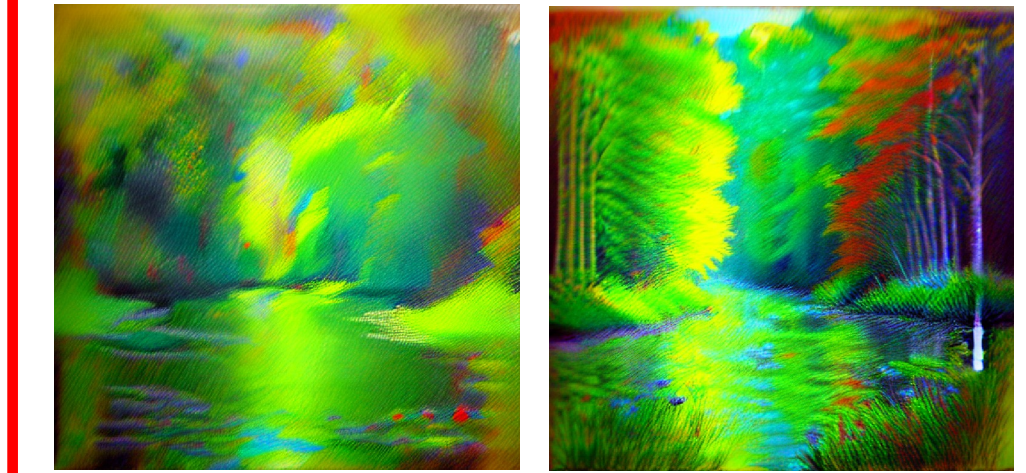

Prompt: 'a painting of a forest'

PDM-Pure

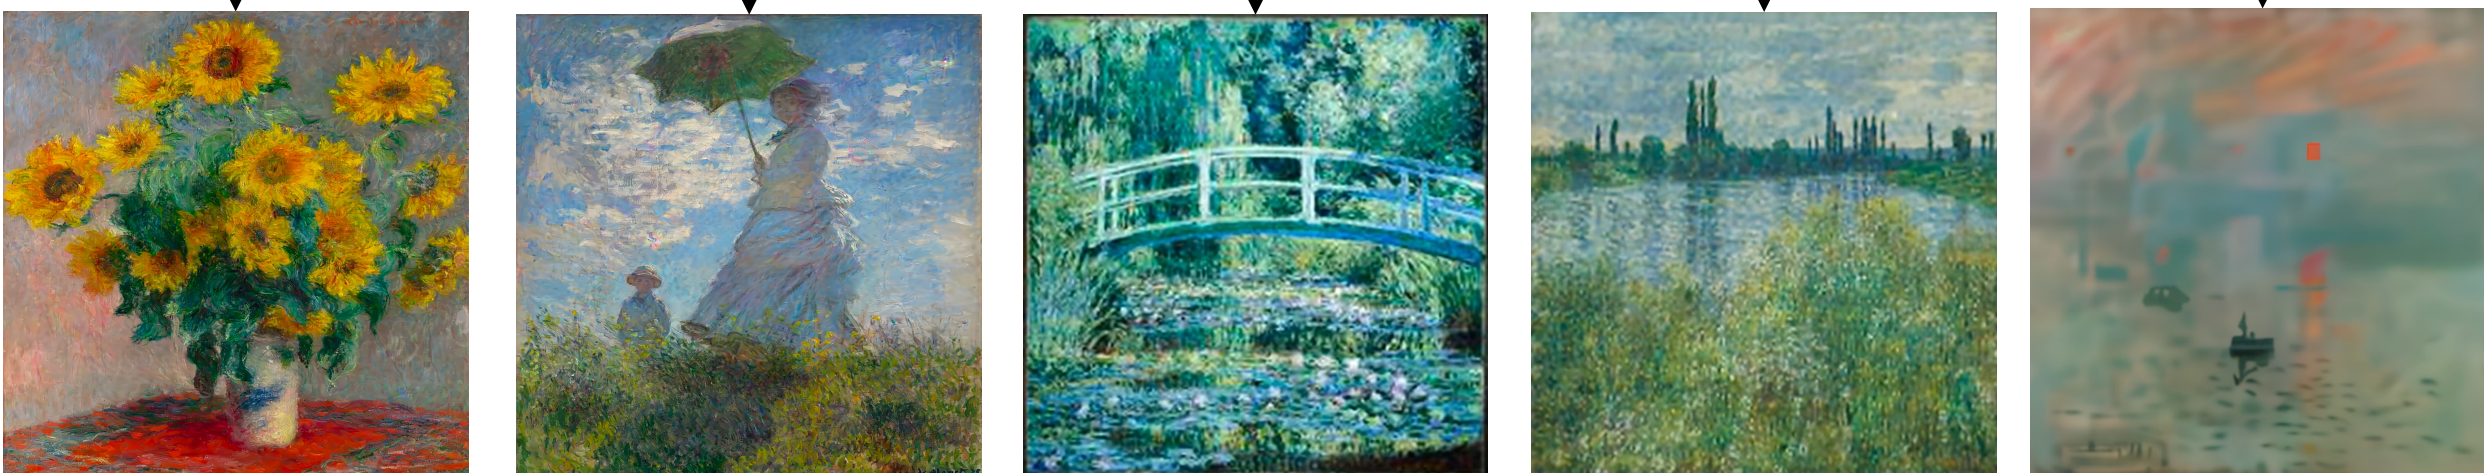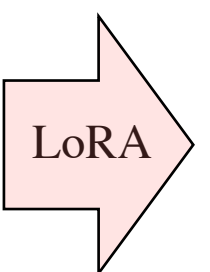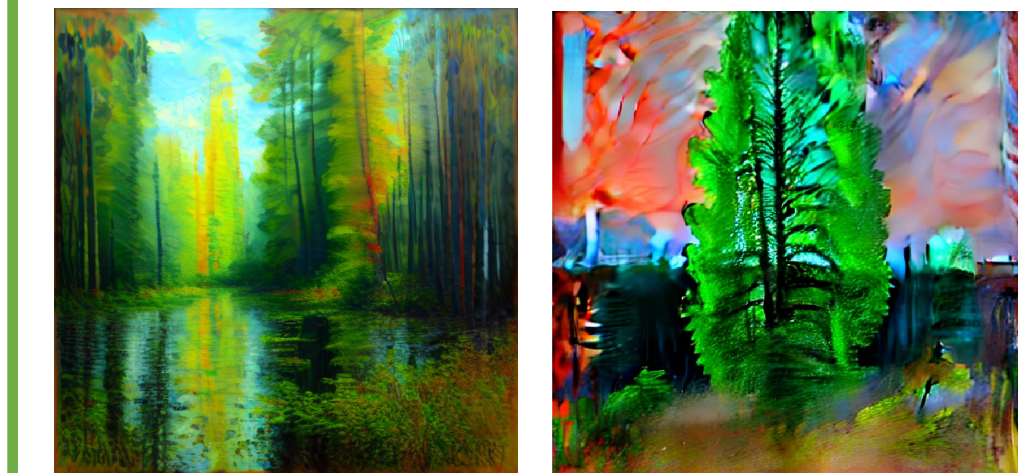

Prompt: 'a painting of a forest'
